# Supplementary material for: First observations of $h_c \to$ hadrons
Source: arXiv:1810.12023 source file (2019-05-17)
Supplement: Supplementary file 1 [file supplemental.pdf]

# Supplemental Material for "First Observations of $h_c \rightarrow$hadrons"

M. Ablikim[1], M. N. Achasov[10,d], S. Ahmed[15], M. Albrecht[4], M. Alekseev[55A,55C], A. Amoroso[55A,55C], F. F. An[1], Q. An[52,42], J. Z. Bai[1], Y. Bai[41], O. Bakina[27], R. Baldini Ferroli[23A], Y. Ban[35], K. Begzsuren[25], D. W. Bennett[22], J. V. Bennett[5], N. Berger[26], M. Bertani[23A], D. Bettoni[24A], F. Bianchi[55A,55C], E. Boger[27,b], I. Boyko[27], R. A. Briere[5], H. Cai[57], X. Cai[1,42], O. Cakir[45A], A. Calcaterra[23A], G. F. Cao[1,46], S. A. Cetin[45B], J. Chai[55C], J. F. Chang[1,42], G. Chelkov[27,b,c], G. Chen[1], H. S. Chen[1,46], J. C. Chen[1], M. L. Chen[1,42], P. L. Chen[53], S. J. Chen[33], X. R. Chen[30], Y. B. Chen[1,42], W. Cheng[55C], X. K. Chu[35], G. Cibinetto[24A], F. Cossio[55C], H. L. Dai[1,42], J. P. Dai[37,h], A. Dbeyssi[15], D. Dedovich[27], Z. Y. Deng[1], A. Denig[26], I. Denysenko[27], M. Destefanis[55A,55C], F. De Mori[55A,55C], Y. Ding[31], C. Dong[34], J. Dong[1,42], L. Y. Dong[1,46], M. Y. Dong[1,42,46], Z. L. Dou[33], S. X. Du[60], P. F. Duan[1], J. Fang[1,42], S. S. Fang[1,46], Y. Fang[1], R. Farinelli[24A,24B], L. Fava[55B,55C], S. Fegan[26], F. Feldbauer[4], G. Felici[23A], C. Q. Feng[52,42], E. Fioravanti[24A], M. Fritsch[4], C. D. Fu[1], Q. Gao[1], X. L. Gao[52,42], Y. Gao[44], Y. G. Gao[6], Z. Gao[52,42], B. Garillon[26], I. Garzia[24A], A. Gilman[49], K. Goetzen[11], L. Gong[34], W. X. Gong[1,42], W. Gradl[26], M. Greco[55A,55C], L. M. Gu[33], M. H. Gu[1,42], Y. T. Gu[13], A. Q. Guo[1], L. B. Guo[32], R. P. Guo[1,46], Y. P. Guo[26], A. Guskov[27], Z. Haddadi[29], S. Han[57], X. Q. Hao[16], F. A. Harris[47], K. L. He[1,46], X. Q. He[51], F. H. Heinsius[4], T. Held[4], Y. K. Heng[1,42,46], Z. L. Hou[1], H. M. Hu[1,46], J. F. Hu[37,h], T. Hu[1,42,46], Y. Hu[1], G. S. Huang[52,42], J. S. Huang[16], X. T. Huang[36], X. Z. Huang[33], Z. L. Huang[31], T. Hussain[54], W. Ikegami Andersson[56], M, Irshad[52,42], Q. Ji[1], Q. P. Ji[16], X. B. Ji[1,46], X. L. Ji[1,42], X. S. Jiang[1,42,46], X. Y. Jiang[34], J. B. Jiao[36], Z. Jiao[18], D. P. Jin[1,42,46], S. Jin[1,46], Y. Jin[48], T. Johansson[56], A. Julin[49], N. Kalantar-Nayestanaki[29], X. S. Kang[34], M. Kavatsyuk[29], B. C. Ke[1], I. K. Keshk[4], T. Khan[52,42], A. Khoukaz[50], P. Kiese[26], R. Kiuchi[1], R. Kliemt[11], L. Koch[28], O. B. Kolcu[45B,f], B. Kopf[4], M. Kornicer[47], M. Kuemmel[4], M. Kuessner[4], A. Kupsc[56], M. Kurth[1], W. Kühn[28], J. S. Lange[28], P. Larin[15], L. Lavezzi[55C], S. Leiber[4], H. Leithoff[26], C. Li[56], Cheng Li[52,42], D. M. Li[60], F. Li[1,42], F. Y. Li[35], G. Li[1], H. B. Li[1,46], H. J. Li[1,46], J. C. Li[1], J. W. Li[40], K. J. Li[43], Kang Li[14], Ke Li[1], Lei Li[3], P. L. Li[52,42], P. R. Li[46,7], Q. Y. Li[36], T. Li[36], W. D. Li[1,46], W. G. Li[1], X. L. Li[36], X. N. Li[1,42], X. Q. Li[34], Z. B. Li[43], H. Liang[52,42], Y. F. Liang[39], Y. T. Liang[28], G. R. Liao[12], L. Z. Liao[1,46], J. Libby[21], C. X. Lin[43], D. X. Lin[15], B. Liu[37,h], B. J. Liu[1], C. X. Liu[1], D. Liu[52,42], D. Y. Liu[37,h], F. H. Liu[38], Fang Liu[1], Feng Liu[6], H. B. Liu[13], H L Liu[41], H. M. Liu[1,46], Huanhuan Liu[1], Huihui Liu[17], J. B. Liu[52,42], J. Y. Liu[1,46], K. Liu[44], K. Y. Liu[31], Ke Liu[6], L. D. Liu[35], Q. Liu[46], S. B. Liu[52,42], X. Liu[30], Y. B. Liu[34], Z. A. Liu[1,42,46], Zhiqing Liu[26], Y. F. Long[35], X. C. Lou[1,42,46], H. J. Lu[18], J. G. Lu[1,42], Y. Lu[1], Y. P. Lu[1,42], C. L. Luo[32], M. X. Luo[59], T. Luo[9,j], X. L. Luo[1,42], S. Lusso[55C], X. R. Lyu[46], F. C. Ma[31], H. L. Ma[1], L. L. Ma[36], M. M. Ma[1,46], Q. M. Ma[1], T. Ma[1], X. N. Ma[34], X. Y. Ma[1,42], Y. M. Ma[36], F. E. Maas[15], M. Maggiora[55A,55C], S. Maldaner[26], Q. A. Malik[54], A. Mangoni[23B], Y. J. Mao[35], Z. P. Mao[1], S. Marcello[55A,55C], Z. X. Meng[48], J. G. Messchendorp[29], G. Mezzadri[24B], J. Min[1,42], T. J. Min[33], R. E. Mitchell[22], X. H. Mo[1,42,46], Y. J. Mo[6], C. Morales Morales[15], N. Yu. Muchnoi[10,d], H. Muramatsu[49], A. Mustafa[4], Y. Nefedov[27], F. Nerling[11], I. B. Nikolaev[10,d], Z. Ning[1,42], S. Nisar[8], S. L. Niu[1,42], X. Y. Niu[1,46], S. L. Olsen[46], Q. Ouyang[1,42,46], S. Pacetti[23B], Y. Pan[52,42], M. Papenbrock[56], P. Patteri[23A], M. Pelizaeus[4], J. Pellegrino[55A,55C], H. P. Peng[52,42], Z. Y. Peng[13], K. Peters[11,g], J. Pettersson[56], J. L. Ping[32], R. G. Ping[1,46], A. Pitka[4], R. Poling[49], V. Prasad[52,42], H. R. Qi[2], M. Qi[33], T. Y. Qi[2], S. Qian[1,42], C. F. Qiao[46], N. Qin[57], X. S. Qin[4], Z. H. Qin[1,42], J. F. Qiu[1], S. Q. Qu[34], K. H. Rashid[54,i], C. F. Redmer[26], M. Richter[4], M. Ripka[26], A. Rivetti[55C], M. Rolo[55C], G. Rong[1,46], Ch. Rosner[15], A. Sarantsev[27,e], M. Savrié[24B], K. Schoenning[56], W. Shan[19], X. Y. Shan[52,42], M. Shao[52,42], C. P. Shen[2], P. X. Shen[34], X. Y. Shen[1,46], H. Y. Sheng[1], X. Shi[1,42], J. J. Song[36], W. M. Song[36], X. Y. Song[1], S. Sosio[55A,55C], C. Sowa[4], S. Spataro[55A,55C], G. X. Sun[1], J. F. Sun[16], L. Sun[57], S. S. Sun[1,46], X. H. Sun[1], Y. J. Sun[52,42], Y. K Sun[52,42], Y. Z. Sun[1], Z. J. Sun[1,42], Z. T. Sun[1], Y. T Tan[52,42], C. J. Tang[39], G. Y. Tang[1], X. Tang[1], I. Tapan[45C], M. Tiemens[29], B. Tsednee[25], I. Uman[45D], B. Wang[1], B. L. Wang[46], C. W. Wang[33], D. Wang[35], D. Y. Wang[35], Dan Wang[46], K. Wang[1,42], L. L. Wang[1], L. S. Wang[1], M. Wang[36], Meng Wang[1,46], P. Wang[1], P. L. Wang[1], W. P. Wang[52,42], X. F. Wang[44], Y. Wang[52,42], Y. F. Wang[1,42,46], Z. Wang[1,42], Z. G. Wang[1,42], Z. Y. Wang[1], Zongyuan Wang[1,46], T. Weber[4], D. H. Wei[12], P. Weidenkaff[26], S. P. Wen[1], U. Wiedner[4], M. Wolke[56], L. H. Wu[1], L. J. Wu[1,46], Z. Wu[1,42], L. Xia[52,42], X. Xia[36], Y. Xia[20], D. Xiao[1], Y. J. Xiao[1,46], Z. J. Xiao[32], Y. G. Xie[1,42], Y. H. Xie[6], X. A. Xiong[1,46], Q. L. Xiu[1,42], G. F. Xu[1], J. J. Xu[1,46], L. Xu[1], Q. J. Xu[14], Q. N. Xu[46], X. P. Xu[40], F. Yan[53], L. Yan[55A,55C], W. B. Yan[52,42], W. C. Yan[2], Y. H. Yan[20], H. J. Yang[37,h], H. X. Yang[1], L. Yang[57], R. X. Yang[52,42], Y. H. Yang[33], Y. X. Yang[12], Yifan Yang[1,46], Z. Q. Yang[20], M. Ye[1,42], M. H. Ye[7], J. H. Yin[1], Z. Y. You[43], B. X. Yu[1,42,46], C. X. Yu[34], J. S. Yu[30], J. S. Yu[20], C. Z. Yuan[1,46], Y. Yuan[1], A. Yuncu[45B,a], A. A. Zafar[54], Y. Zeng[20], B. X. Zhang[1], B. Y. Zhang[1,42], C. C. Zhang[1], D. H. Zhang[1], H. H. Zhang[43], H. Y. Zhang[1,42], J. Zhang[1,46], J. L. Zhang[58], J. Q. Zhang[4], J. W. Zhang[1,42,46], J. Y. Zhang[1], J. Z. Zhang[1,46], K. Zhang[1,46], L. Zhang[44], S. F. Zhang[33], T. J. Zhang[37,h], X. Y. Zhang[36], Y. Zhang[52,42], Y. H. Zhang[1,42], Y. T. Zhang[52,42], Yang Zhang[1], Yao Zhang[1], Yu Zhang[46], Z. H. Zhang[6], Z. P. Zhang[52], Z. Y. Zhang[57], G. Zhao[1], J. W. Zhao[1,42], J. Y. Zhao[1,46], J. Z. Zhao[1,42],

Typeset by REVTEX

Lei Zhao[52,42], Ling Zhao[1], M. G. Zhao[34], Q. Zhao[1], S. J. Zhao[60], T. C. Zhao[1], Y. B. Zhao[1,42], Z. G. Zhao[52,42], A. Zhemchugov[27,b], B. Zheng[53], J. P. Zheng[1,42], W. J. Zheng[36], Y. H. Zheng[46], B. Zhong[32], L. Zhou[1,42], Q. Zhou[1,46], X. Zhou[57], X. K. Zhou[52,42], X. R. Zhou[52,42], X. Y. Zhou[1], Xiaoyu Zhou[20], Xu Zhou[20], A. N. Zhu[1,46], J. Zhu[34], J. Zhu[43], K. Zhu[1], K. J. Zhu[1,42,46], S. Zhu[1], S. H. Zhu[51], X. L. Zhu[44], Y. C. Zhu[52,42], Y. S. Zhu[1,46], Z. A. Zhu[1,46], J. Zhuang[1,42], B. S. Zou[1], J. H. Zou[1]

(BESIII Collaboration)

[1] *Institute of High Energy Physics, Beijing 100049, People's Republic of China*
[2] *Beihang University, Beijing 100191, People's Republic of China*
[3] *Beijing Institute of Petrochemical Technology, Beijing 102617, People's Republic of China*
[4] *Bochum Ruhr-University, D-44780 Bochum, Germany*
[5] *Carnegie Mellon University, Pittsburgh, Pennsylvania 15213, USA*
[6] *Central China Normal University, Wuhan 430079, People's Republic of China*
[7] *China Center of Advanced Science and Technology, Beijing 100190, People's Republic of China*
[8] *COMSATS Institute of Information Technology, Lahore, Defence Road, Off Raiwind Road, 54000 Lahore, Pakistan*
[9] *Fudan University, Shanghai 200443, People's Republic of China*
[10] *G.I. Budker Institute of Nuclear Physics SB RAS (BINP), Novosibirsk 630090, Russia*
[11] *GSI Helmholtzcentre for Heavy Ion Research GmbH, D-64291 Darmstadt, Germany*
[12] *Guangxi Normal University, Guilin 541004, People's Republic of China*
[13] *Guangxi University, Nanning 530004, People's Republic of China*
[14] *Hangzhou Normal University, Hangzhou 310036, People's Republic of China*
[15] *Helmholtz Institute Mainz, Johann-Joachim-Becher-Weg 45, D-55099 Mainz, Germany*
[16] *Henan Normal University, Xinxiang 453007, People's Republic of China*
[17] *Henan University of Science and Technology, Luoyang 471003, People's Republic of China*
[18] *Huangshan College, Huangshan 245000, People's Republic of China*
[19] *Hunan Normal University, Changsha 410081, People's Republic of China*
[20] *Hunan University, Changsha 410082, People's Republic of China*
[21] *Indian Institute of Technology Madras, Chennai 600036, India*
[22] *Indiana University, Bloomington, Indiana 47405, USA*
[23] *(A)INFN Laboratori Nazionali di Frascati, I-00044, Frascati, Italy; (B)INFN and University of Perugia, I-06100, Perugia, Italy*
[24] *(A)INFN Sezione di Ferrara, I-44122, Ferrara, Italy; (B)University of Ferrara, I-44122, Ferrara, Italy*
[25] *Institute of Physics and Technology, Peace Ave. 54B, Ulaanbaatar 13330, Mongolia*
[26] *Johannes Gutenberg University of Mainz, Johann-Joachim-Becher-Weg 45, D-55099 Mainz, Germany*
[27] *Joint Institute for Nuclear Research, 141980 Dubna, Moscow region, Russia*
[28] *Justus-Liebig-Universitaet Giessen, II. Physikalisches Institut, Heinrich-Buff-Ring 16, D-35392 Giessen, Germany*
[29] *KVI-CART, University of Groningen, NL-9747 AA Groningen, The Netherlands*
[30] *Lanzhou University, Lanzhou 730000, People's Republic of China*
[31] *Liaoning University, Shenyang 110036, People's Republic of China*
[32] *Nanjing Normal University, Nanjing 210023, People's Republic of China*
[33] *Nanjing University, Nanjing 210093, People's Republic of China*
[34] *Nankai University, Tianjin 300071, People's Republic of China*
[35] *Peking University, Beijing 100871, People's Republic of China*
[36] *Shandong University, Jinan 250100, People's Republic of China*
[37] *Shanghai Jiao Tong University, Shanghai 200240, People's Republic of China*
[38] *Shanxi University, Taiyuan 030006, People's Republic of China*
[39] *Sichuan University, Chengdu 610064, People's Republic of China*
[40] *Soochow University, Suzhou 215006, People's Republic of China*
[41] *Southeast University, Nanjing 211100, People's Republic of China*
[42] *State Key Laboratory of Particle Detection and Electronics, Beijing 100049, Hefei 230026, People's Republic of China*
[43] *Sun Yat-Sen University, Guangzhou 510275, People's Republic of China*
[44] *Tsinghua University, Beijing 100084, People's Republic of China*

[45] *(A)Ankara University, 06100 Tandogan, Ankara, Turkey; (B)Istanbul Bilgi University, 34060 Eyup, Istanbul, Turkey; (C)Uludag University, 16059 Bursa, Turkey; (D)Near East University, Nicosia, North Cyprus, Mersin 10, Turkey*
[46] *University of Chinese Academy of Sciences, Beijing 100049, People's Republic of China*
[47] *University of Hawaii, Honolulu, Hawaii 96822, USA*
[48] *University of Jinan, Jinan 250022, People's Republic of China*
[49] *University of Minnesota, Minneapolis, Minnesota 55455, USA*
[50] *University of Muenster, Wilhelm-Klemm-Str. 9, 48149 Muenster, Germany*
[51] *University of Science and Technology Liaoning, Anshan 114051, People's Republic of China*
[52] *University of Science and Technology of China, Hefei 230026, People's Republic of China*
[53] *University of South China, Hengyang 421001, People's Republic of China*
[54] *University of the Punjab, Lahore-54590, Pakistan*
[55] *(A)University of Turin, I-10125, Turin, Italy; (B)University of Eastern Piedmont, I-15121, Alessandria, Italy; (C)INFN, I-10125, Turin, Italy*
[56] *Uppsala University, Box 516, SE-75120 Uppsala, Sweden*
[57] *Wuhan University, Wuhan 430072, People's Republic of China*
[58] *Xinyang Normal University, Xinyang 464000, People's Republic of China*
[59] *Zhejiang University, Hangzhou 310027, People's Republic of China*
[60] *Zhengzhou University, Zhengzhou 450001, People's Republic of China*

[a] *Also at Bogazici University, 34342 Istanbul, Turkey*
[b] *Also at the Moscow Institute of Physics and Technology, Moscow 141700, Russia*
[c] *Also at the Functional Electronics Laboratory, Tomsk State University, Tomsk, 634050, Russia*
[d] *Also at the Novosibirsk State University, Novosibirsk, 630090, Russia*
[e] *Also at the NRC "Kurchatov Institute", PNPI, 188300, Gatchina, Russia*
[f] *Also at Istanbul Arel University, 34295 Istanbul, Turkey*
[g] *Also at Goethe University Frankfurt, 60323 Frankfurt am Main, Germany*
[h] *Also at Key Laboratory for Particle Physics, Astrophysics and Cosmology, Ministry of Education; Shanghai Key Laboratory for Particle Physics and Cosmology; Institute of Nuclear and Particle Physics, Shanghai 200240, People's Republic of China*
[i] *Government College Women University, Sialkot - 51310. Punjab, Pakistan.*
[j] *Key Laboratory of Nuclear Physics and Ion-beam Application (MOE) and Institute of Modern Physics, Fudan University, Shanghai 200443, People's Republic of China*

(Dated: January 2, 2019)

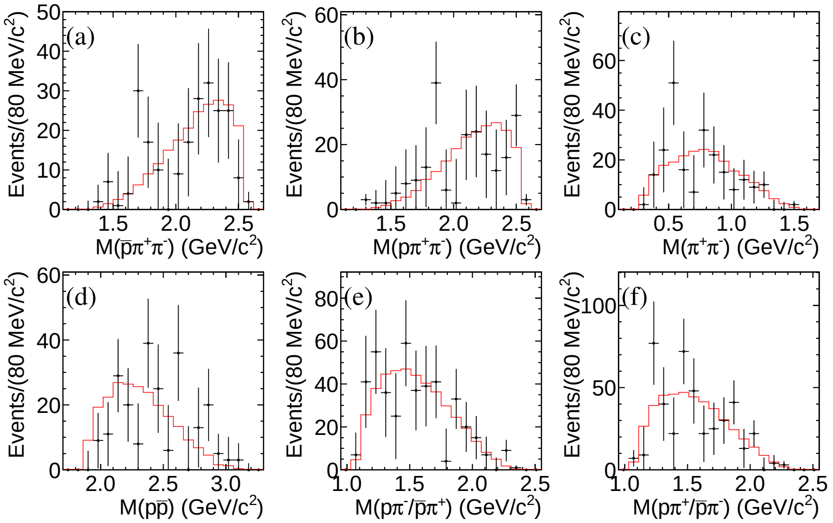


FIG. 1. The invariant mass spectra of (a) $\bar{p}\pi^+\pi^-$, (b) $p\pi^+\pi^-$, (c) $\pi^+\pi^-$, (d)$p\bar{p}$, (e) $p\pi^-/\bar{p}\pi^+$, and (f) $p\pi^+/\bar{p}\pi^-$ for decay mode $h_c \to p\bar{p}\pi^+\pi^-$. In each spectra, the dots are data subtracted sideband background, the red histogram is the PHSP signal MC (color online).

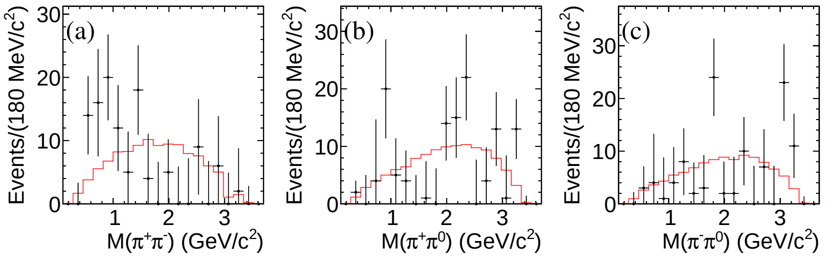


FIG. 2. The invariant mass spectra of (a) $\pi^+\pi^-$, (b) $\pi^+\pi^0$, and (c) $\pi^-\pi^0$ for decay mode $h_c \to \pi^+\pi^-\pi^0$. In each spectra, the dots are data subtracted sideband background, the red histogram is the PHSP signal MC (color online).

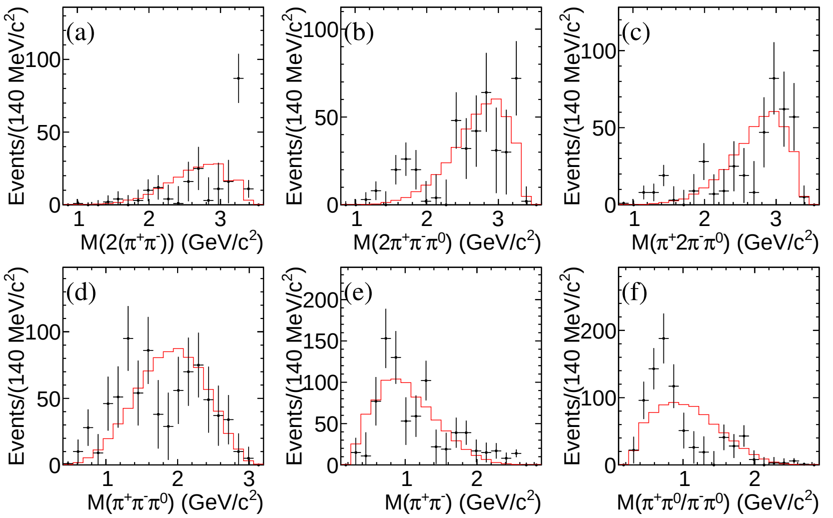


FIG. 3. The invariant mass spectra of (a) $2(\pi^+\pi^-)$, (b) $2\pi^+\pi^-\pi^0$, (c) $\pi^+2\pi^-\pi^0$, (d) $\pi^+\pi^-\pi^0$, (e) $\pi^+\pi^-$, and (f) $\pi^+\pi^0/\pi^-\pi^0$ for decay mode $h_c \to 2(\pi^+\pi^-)\pi^0$. In each spectra, the dots are data subtracted sideband background, the red histogram is PHSP signal MC (color online).
